# Supplementary material for: Tuning Multigrid Methods with Robust Optimization
Source: arXiv:2001.00887 source file (2020-07-27)
Supplement: Supplementary file 1 [file supp.pdf]

**1. LFA Symbols.** For convenience, we summarize here the Fourier symbols used throughout this work.

**1.1. Poisson.** For factor-two coarsening, the symbols for the one-dimensional P1 Poisson operator are given in Section 4.3. For coarsening-by-three multigrid of the same problem, the interpolation symbol is

$$\tilde{\mathbf{P}}_h = \frac{1}{3} \begin{pmatrix} 1 + 2 \cos(\theta) \\ 1 + 2 \cos\left(\theta + \frac{2\pi}{3}\right) \\ 1 + 2 \cos\left(\theta + \frac{4\pi}{3}\right) \end{pmatrix},$$

with  $\tilde{\mathbf{R}}_h = 3\tilde{\mathbf{P}}_h^T$ . Here, the symbol for the coarse-grid operator is given by

$$I - \tilde{\mathbf{P}}_h \left( \tilde{L}_H(3\theta) \right)^{-1} \tilde{\mathbf{R}}_h(\theta) \tilde{\mathcal{L}}_h(\theta),$$

where  $H = 3h$ , and  $\tilde{\mathcal{L}}_h$  is the  $3 \times 3$  diagonal matrix with entries given by  $\tilde{L}_h$  evaluated at frequencies  $\theta \in [-\frac{\pi}{3}, \frac{\pi}{3})$ ,  $\theta + \frac{2\pi}{3}$ , and  $\theta + \frac{4\pi}{3}$ .  $\tilde{\mathbf{S}}_h$  is defined similarly.

For the P2 discretization of the 2D problem, the  $4 \times 4$  symbol for the operator is given in Section 3.3 of [?]. The symbol for the restriction operator is given in Section 3.4 of [?], with  $\tilde{\mathbf{P}}_h = \frac{1}{4}\tilde{\mathbf{R}}_h^T$ . We consider weighted Jacobi relaxation, with error-propagation operator given by  $I - p_1 M_h^{-1} L_h$ . The symbol for  $M_h$  is given by

$$\tilde{M}_h = \frac{1}{3} \begin{pmatrix} 12 & 0 & 0 & 0 \\ 0 & 16 & 0 & 0 \\ 0 & 0 & 16 & 0 \\ 0 & 0 & 0 & 16 \end{pmatrix}.$$

**1.2. Stokes Equations.** Local Fourier analysis for the MAC-scheme finite-difference discretization of the Stokes equations is given in [?]. The  $3 \times 3$  symbol for  $L_h$  is given in Section 2.2, the symbol for the inexact Braess-Sarazin relaxation scheme is given in Section 4.3, and the symbol for the Uzawa relaxation scheme is given in Section 5.2. That paper focuses on LFA smoothing analysis, so does not present symbols for the interpolation and restriction operators used. Below, we give the details of these grid-transfer operators and their symbols. We consider block-structured restriction and interpolation operators,

$$R_h = \begin{pmatrix} R_u & 0 & 0 \\ 0 & R_v & 0 \\ 0 & 0 & R_p \end{pmatrix} \text{ and } P_h = \begin{pmatrix} P_u & 0 & 0 \\ 0 & P_v & 0 \\ 0 & 0 & P_p \end{pmatrix},$$

where  $R_u$  and  $R_v$  ( $P_u$  and  $P_v$ ) are the restriction (interpolation) operators for the two components of the velocity vector and  $R_p$  ( $P_p$ ) is the restriction (interpolation) operator for the pressure. As explained in Section 2.1, the block symbols of  $R_h$  and  $P_h$  are composed row/column-wise from their symbols evaluated at each of the four frequencies in a harmonic set (in 2D). Here, we give the formula for each harmonic frequency.

They are many possible choices for these grid-transfer operators, see [?]. We consider  $R_u$  to be the (scaled) transpose of bilinear interpolation, which uses 12 points

33 on the staggered mesh, with stencil

$$34 \quad R_u = \frac{1}{32} \begin{bmatrix} 1 & 2 & 1 \\ 3 & 6 & 3 \\ & \cdot & \\ 3 & 6 & 3 \\ 1 & 2 & 1 \end{bmatrix},$$

35 where the  $\cdot$  denotes the position on the coarse grid at which the restriction is applied,  
36 and  $P_u = 4R_u^T$ . The symbols are

$$37 \quad \tilde{R}_u(\boldsymbol{\theta}^\alpha) = (-1)^{\alpha_2} \cos(\theta_1^{\alpha_1}/2)^2 \cos(\theta_2^{\alpha_2}/2)^3, \quad \tilde{P}_u(\boldsymbol{\theta}^\alpha) = \tilde{R}_u^T(\boldsymbol{\theta}^\alpha).$$

38 For  $R_v$ , we again consider the (scaled) transpose of bilinear interpolation, whose  
39 stencil is a  $90^\circ$  rotation of that of  $R_u$ , and whose symbol is, then,

$$40 \quad \tilde{R}_v(\boldsymbol{\theta}^\alpha) = (-1)^{\alpha_1} \cos(\theta_1^{\alpha_1}/2)^3 \cos(\theta_2^{\alpha_2}/2)^2.$$

41 For  $P_v$ , we use the 6-point stencil given by

$$42 \quad P_v = \frac{1}{2} \begin{bmatrix} & & & & & \\ & & & & & \\ & & & & & \\ & & & & & \\ & & & & & \\ & & & & & \end{bmatrix} \begin{matrix} 1 & 2 & 1 \\ & \cdot & \\ 1 & 2 & 1 \end{matrix} \begin{matrix} \uparrow^h \\ \\ \downarrow_{2h} \end{matrix},$$

43 where the  $\cdot$  denotes the position on the fine grid to which the interpolation maps,  
44 with symbol

$$45 \quad \tilde{P}_v(\boldsymbol{\theta}^\alpha) = (-1)^{\alpha_1} \cos(\theta_1^{\alpha_1}/2) \cos(\theta_2^{\alpha_2}/2)^2.$$

46 For the pressure,  $R_p$  is the standard four-point (cell-centred) restriction operator,  
47 with stencil

$$48 \quad R_p = \frac{1}{4} \begin{bmatrix} 1 & & 1 \\ & \cdot & \\ 1 & & 1 \end{bmatrix}$$

49 and  $P_p = 4R_p^T$ . The symbols are given by

$$50 \quad \tilde{R}_p(\boldsymbol{\theta}^\alpha) = (-1)^{\alpha_1 + \alpha_2} \cos(\theta_1^{\alpha_1}/2) \cos(\theta_2^{\alpha_2}/2), \quad \tilde{P}_p(\boldsymbol{\theta}^\alpha) = \tilde{R}_p^T(\boldsymbol{\theta}^\alpha).$$

51 LFA for the stabilized Q1-Q1 discretization of the Stokes equations is given in [?].  
52 The  $3 \times 3$  symbol for  $L_h$  is given in Section 3.2.1, and the symbol for distributive  
53 weighted-Jacobi relaxation is given in Section 4.1. The symbols for interpolation  
54 and restriction for Q1 finite elements are classical, and can be found, for example,  
55 in [?, Section 4.4].

56 LFA for the P2-P1 discretization of the Stokes equations is given in [?]. The  $9 \times 9$   
57 symbol for  $L_h$  is given in Section 3.3, the symbols for the grid-transfer operators are  
58 given in Section 3.4, and the symbols for the additive Vanka relaxation scheme are  
59 given in Section 3.6.

**1.3. Control Problem.** For the 3D elliptic optimal control problem in Section 4.5, the symbol of  $\mathcal{A}$  at a single frequency is a  $3 \times 3$  matrix given by

$$\tilde{\mathcal{A}}(\boldsymbol{\theta}^\alpha) = \begin{pmatrix} \tilde{M}(\boldsymbol{\theta}^\alpha) & \tilde{K}^T(\boldsymbol{\theta}^\alpha) & 0 \\ \tilde{K}(\boldsymbol{\theta}^\alpha) & 0 & -\tilde{M}(\boldsymbol{\theta}^\alpha) \\ 0 & -\tilde{M}^T(\boldsymbol{\theta}^\alpha) & \beta \tilde{M}(\boldsymbol{\theta}^\alpha) \end{pmatrix},$$

where

$$\tilde{K}(\boldsymbol{\theta}^\alpha) = \frac{2h(4 - \cos \theta_1^{\alpha_1} \cos \theta_2^{\alpha_2} - \cos \theta_1^{\alpha_1} \cos \theta_3^{\alpha_3} - (1 + \cos \theta_1^{\alpha_1})(\cos \theta_2^{\alpha_2} \cos \theta_3^{\alpha_3}))}{3},$$

and

$$\tilde{M}(\boldsymbol{\theta}^\alpha) = \frac{h^3}{27}(4 + 2 \cos \theta_1^{\alpha_1} + 2 \cos \theta_2^{\alpha_2} + \cos \theta_1^{\alpha_1} \cos \theta_2^{\alpha_2})(2 + \cos \theta_3^{\alpha_3}),$$

are the symbols of the Q1 stiffness and mass matrices in 3D, respectively. We consider the weighted block-Jacobi relaxation scheme,  $\mathcal{S}_h = I - p_1 \hat{\mathcal{A}}^{-1} \mathcal{A}$ , and the symbol of  $\hat{\mathcal{A}}$  is given by

$$\hat{\mathcal{A}}(\boldsymbol{\theta}^\alpha) = \begin{pmatrix} \frac{8h^3}{27} & p_2 \frac{8h}{3} & 0 \\ p_2 \frac{8h}{3} & 0 & -\frac{8h^3}{27} \\ 0 & -\frac{8h^3}{27} & \beta \frac{8h^3}{27} \end{pmatrix}.$$

Each of these is sampled at the 8 frequencies within a harmonic set to yield the  $24 \times 24$  matrix that is the symbol for relaxation, which is block diagonal with  $3 \times 3$  diagonal blocks. We use independent trilinear interpolation and restriction operators for each component of the system, leading to symbols for each harmonic frequency that are diagonal with the equal diagonal entries given by

$$\tilde{P}_h(\boldsymbol{\theta}^\alpha) = \frac{1}{8} \prod_{j=1}^3 (1 + \cos(\theta_j^{\alpha_j})) \text{ and } \tilde{R}_h(\boldsymbol{\theta}^\alpha) = \prod_{j=1}^3 (1 + \cos(\theta_j^{\alpha_j})).$$

**2. Software framework.** Our software for this project was written in Matlab. For each example, we have a Matlab script that takes, as input, values for a Fourier frequency  $\boldsymbol{\theta} \in T^{\text{low}}$  and parameters  $\mathbf{p}$ , as well as possible additional inputs to specify a choice of relaxation scheme or step-size for a finite-difference derivative approximation, and returns, as output, the value of the spectral radius of the Fourier symbol at frequency  $\boldsymbol{\theta}$  and parameters  $\mathbf{p}$ . Optionally, it also returns a (sub-)gradient of the spectral radius, evaluated either analytically or through finite-differencing. Additionally, these routines increment global counters for function evaluations and other diagnostic information.

In what follows below, we refer to such as routine as `symbol(x,u,opts)`, where  $\mathbf{x}$  is the parameter variable (corresponding to  $\mathbf{p}$ ),  $\mathbf{u}$  is the frequency variable (corresponding to  $\boldsymbol{\theta}$ , also called the uncertainty set), and `opts` refers to any other options to be passed to the routine that computes the symbol and its spectral radius. Canonically, we take  $\mathbf{n}$  to be the dimension of the parameter variable and  $\mathbf{m}$  to be the dimension of the frequency variable.

To interface with HANSO, we wrap the problem with two data structures, `pars` and `opts`, prescribed by the HANSO code. Within `pars`, we set the number of optimization variables,  $\mathbf{n}$ , and give the name to a wrapper function (`hanso_wrapper`)

that encapsulates the inner discretization on a fixed mesh. We change only two of the default HANSO options in `opts`, setting the initial guess (as discussed Section 4.1) to have  $p_i = 0.5$  for all  $i$  (or  $p_i = 0.1$  for the Laplacian examples) and to adjust the maximum number of iterations to account for a fixed computational budget of symbol evaluations. Thus, our calls to HANSO take the form

```

100 problem.objective = @(x,u)symbol(x,u,opts);
101 x0 = 0.5*ones(n,1);
102
103
104 pars.resolution = 32;
105 pars.nvar = n;
106 pars.fgname = 'hanso-wrapper';
107 opts.x0 = x0;
108 opts.maxit = floor(budget/(2*pars.resolution^m));
109 [x_Hanso,f] = hanso(pars,opts);

```

while `hanso_wrapper` for a two-dimensional Fourier space takes the form

```

112 function [f,g] = hanso_wrapper(x,pars)
113
114 global problem
115
116 func_f = problem.objective;
117 resolution = pars.resolution;
118 n = length(x);
119
120 Z = zeros(resolution);
121
122 theta1 = linspace(-pi/2,pi/2,resolution);
123 theta2 = linspace(-pi/2,pi/2,resolution);
124 for i = 1:resolution
125     for j = 1:resolution
126         try
127             [Z(i,j),g] = func_f(x,[theta1(i);theta2(j)]);
128         catch
129             [Z(i,j),g] = func_f(x,[0;0]);
130         end
131     end
132 end
133
134 % return Psi value:
135 f = max(max(Z));
136
137 % return a unique associated subgradient:
138 maxind = find(Z == max(Z(:)));
139 if nargout >= 2
140     Id_row = mod(maxind(1),resolution);
141
142     if Id_row==0 %% deal with the special case
143         Id_row = resolution;
144         Id_column = maxind(1)/resolution;
145     end

```

```

146     else
147         Id_column = fix(maxind(1)/resolution)+1;
148     end
149
150     theta_M1 = theta1(Id_row);
151     theta_M2 = theta2(Id_column);
152     [Z_max,g] = func_f(x,[theta_M1;theta_M2]);
153 end
154

```

155       Calls to ROBBOA again use primarily default parameters, with a typical call  
156 (for a two-dimensional Fourier space) as

```

157
158 problem.lb = [-pi/2;-pi/2]; % lb for uncertainty set
159 problem.ub = [pi/2;pi/2]; % ub for uncertainty set
160 problem.objective = @(x,u)symbol(x,u,opts);
161 x0 = 0.5*ones(n,1);
162
163 U0 = {};
164 Ustruct.u = [0;0];
165 Ustruct.active = 1;
166 U0 = cat(1,U0,Ustruct);
167
168 phase2 = 'general-evp';
169
170 % Solve with derivatives
171 [x_RoboD,XD,UD] = roboboa(problem,x0,U0,phase2,budget,1);
172
173 % Solve with derivative-free methods
174 [x_Robo,X,U] = roboboa(problem,x0,U0,phase2,budget,0);
175

```
